# Supplementary material for: GCondenser: Benchmarking Graph Condensation
Source: arXiv:2405.14246 source file (2024-07-10)
Supplement: Supplementary file 1 [file supp.tex]

\clearpage
\section{Supplementary}
\subsection{Support for Newly Proposed GC Methods}
\texttt{GCondenser} supports newly proposed methods as well, such as GDEM~\cite{liuGraphCondensationEigenbasis2023} and GEOM~\cite{geom}. Due to time constraints, only selected datasets and a limited hyperparameter search are conducted.

Table~\ref{tab:gdem} shows the GDEM condensation performance on relatively smaller graph datasets due to the quadratic time complexity of the Laplacian adjacency matrix decomposition. Table~\ref{tab:geom} shows the GDEM condensation performance on all baseline datasets, with only the GCN backbone utilised due to the time limit.

The results indicate that GDEM and GEOM have the potential to outperform other baseline methods on specific datasets and condensation sizes. However, due to the novelty of these methods and the large number of hyperparameters involved, a thorough parameter search is not feasible to conduct in the limited time available.

\begin{table}[!h]
    \begin{minipage}[t]{0.45\linewidth}
        \centering
        \caption{Results for GDEM method.}
        \tiny
        \label{tab:gdem}
        \begin{tabular}{c|cc|c}\toprule
             Dataset &Size &Ratio &GDEM  \\
             \midrule\midrule
             \multirow{3}{*}{CiteSeer} &30 &0.9\% &71.7 ± 0.3 \\ 
              &60 &1.8\% &72.7 ± 0.6 \\ 
              &120 &3.6\% &73.4 ± 0.4 \\\midrule
             \multirow{3}{*}{Cora} &35 &1.3\% &68.0 ± 0.1 \\ 
              &70 &2.6\% &72.8 ± 0.8 \\ 
              &140 &5.2\% &77.4 ± 0.6 \\\midrule
             \multirow{3}{*}{PubMed} &15 &0.08\% &73.3 ± 0.6 \\ 
              &30 &0.15\% &78.3 ± 0.8 \\ 
              &60 &0.3\% &78.8 ± 0.3 \\\bottomrule
        \end{tabular}
    \end{minipage}\hfill
    \begin{minipage}[t]{0.45\linewidth}
        \centering
        \caption{Results for GEOM method.}
        \tiny
        \label{tab:geom}
        \begin{tabular}{c|ccc|c}\toprule
         Dataset &Backbone &Size &Ratio &GEOM  \\
         \midrule\midrule
         \multirow{3}{*}{CiteSeer} &GCN &30 &0.9\% &69.6 ± 0.6 \\
         &GCN &60 &1.8\% &67.5 ± 0.9 \\
         &GCN &120 &3.6\% &72.1 ± 1.0 \\\midrule
         \multirow{3}{*}{Cora} &GCN &35 &1.3\% &80.3 ± 1.1 \\ 
          &GCN &70 &2.6\% &81.5 ± 0.8 \\ 
          &GCN &140 &5.2\% &82.2 ± 0.4 \\\midrule
         \multirow{3}{*}{PubMed} &GCN &15 &0.08\% &80.1 ± 0.3 \\ 
          &GCN &30 &0.15\% &79.7 ± 0.3 \\ 
          &GCN &60 &0.3\% &79.5 ± 0.4 \\\midrule
          \multirow{3}{*}{Arxiv} &GCN &90 &0.08\% &61.9 ± 0.5 \\ 
          &GCN &454 &0.15\% &65.8 ± 0.4 \\ 
          &GCN &909 &0.3\% &66.2 ± 0.5 \\\midrule
          \multirow{3}{*}{Products} &GCN &612 &0.025\% &68.5 ± 0.3 \\ 
          &GCN &1225 &0.05\% &69.8 ± 0.3 \\ 
          &GCN &2449 &0.1\% &71.1 ± 0.3 \\\midrule\midrule
          \multirow{3}{*}{Flickr} &GCN &44 &0.1\% &44.6 ± 0.5 \\
         &GCN &223 &0.5\% &45.2 ± 0.9 \\
         &GCN &446 &1\% &45.5 ± 0.1 \\\midrule
         \multirow{3}{*}{Reddit} &GCN &153 &0.05\% &90.0 ± 0.5 \\
         &GCN &769 &0.1\% &89.4 ± 0.5 \\
         &GCN &1539 &0.2\% &91.2 ± 0.1 \\\bottomrule
    \end{tabular}
    \end{minipage}
\end{table}
